# Supplementary material for: Iterative Bayesian Learning for Crowdsourced Regression
Source: arXiv:1702.08840 source file (2018-10-08)
Supplement: Supplementary file 1 [file additional_exp.tex]

 % !TEX root =  main.tex

\section{PASCAL Visual Object Classes Datasets (More Results)}
\label{sec:detail_pascal}

\begin{figure*}[t]
\subfigure{
\includegraphics[scale=0.5]{fig/vision/001037avg}%\caption{Average}
}
\subfigure{
\includegraphics[scale=0.5]{fig/vision/001037nav}% \caption{Naive}
}
\subfigure{
\includegraphics[scale=0.5]{fig/vision/001037bp}% \caption{Belief propagation}
}
\subfigure{
\includegraphics[scale=0.5]{fig/vision/001037ora}% \caption{Oracle}
}
\caption{Detection examples on PASCAL VOC2007 test sets. Top left: Average, Top right: Naive, Bottom left: Belief Propagation, Bottom right: Oracles}\label{fig:ex2}
\end{figure*}

%\begin{figure*}[t]
%\centering
%%\includegraphics[width=\textwidth]{figures/001037avg.png}
%\subfigure{
%\includegraphics[scale=0.4]{figures/000547avg.png}%\caption{Average}
%}
%\subfigure{
%\includegraphics[scale=0.4]{figures/000547nav.png}% \caption{Naive}
%}
%\subfigure{
%\includegraphics[scale=0.4]{figures/000547bp.png}% \caption{Belief propagation}
%}
%\subfigure{
%\includegraphics[scale=0.4]{figures/000547ora.png}% \caption{Oracle}
%}
%%\includegraphics[width=\textwidth]{figures/intro_fig_2.png}
%\caption{Detection examples on PASCAL VOC2007 test sets. Top left: Average, Top right: Naive, Bottom left: Belief Propagation, Bottom right: Oracle}\label{fig:ex2}
%\end{figure*}

\begin{figure*}[t]
\subfigure{
\includegraphics[scale=0.5]{fig/vision/000196avg}%\caption{Average}
}
\subfigure{
\includegraphics[scale=0.5]{fig/vision/000196nav}% \caption{Naive}
}
\\
\subfigure{
\includegraphics[scale=0.5]{fig/vision/000196bp}% \caption{Belief propagation}
}
\subfigure{
\includegraphics[scale=0.5]{fig/vision/000196ora}% \caption{Oracle}
}
\caption{Detection examples on PASCAL VOC2007 test sets. Top left: Average, Top right: Naive, Bottom left: Belief Propagation, Bottom right: Oracle}\label{fig:ex3}
\end{figure*}

%%% Local Variables:
%%% mode: latex
%%% TeX-master: "main"
%%% End:
